# Supplementary material for: A Molecular Density Functional Theory of aqueous electrolytic solution
Source: arXiv:2511.09346 ancillary file (2025-11-12)
Supplement: Supplementary file 1 [file SI.pdf]

# Supplementary Informations for: A Molecular Density Functional Theory of aqueous electrolytic solution.

Guillaume Jeanmairet, Luc Belloni and Daniel Borgis

| Atom            | x (Å) | y (Å) | z (Å) | q (e) | $\sigma$ (Å) | $\epsilon$ (kJ/mol) |
|-----------------|-------|-------|-------|-------|--------------|---------------------|
| CH <sub>3</sub> | 1.32  | -1.37 | 0.0   | 0.0   | 3.91         | 0.160               |
| C               | 0.67  | 0.0   | 0.0   | 0.45  | 3.75         | 0.105               |
| O               | 1.31  | 1.01  | 0.0   | -0.45 | 2.96         | 0.210               |
| N               | -0.67 | 0.0   | 0.0   | 0.513 | 3.25         | 0.170               |
| H               | -1.16 | -0.86 | 0.0   | 0.333 | 0.00         | 0.000               |
| CH <sub>3</sub> | -1.43 | 1.23  | 0.0   | 0.18  | 3.80         | 0.170               |

Table I. Position, charge and Lennard-Jones parameters for the NMA solute

## I. STRUCTURE AND FORCE FIELD PARAMETERS USED FOR THE NMA MOLECULE

The position of the atoms and their force field parameters are given in the Table I.

## II. NUMBER AND CHARGE DENSITIES AROUND A NEUTRAL NMA MOLECULE

In figure 1, we display the number densities of chloride and sodium and the charge density in the plane of the NMA molecule which charges have been set to zero. As opposed to the densities of the main article, here there are no electrostatic interaction.

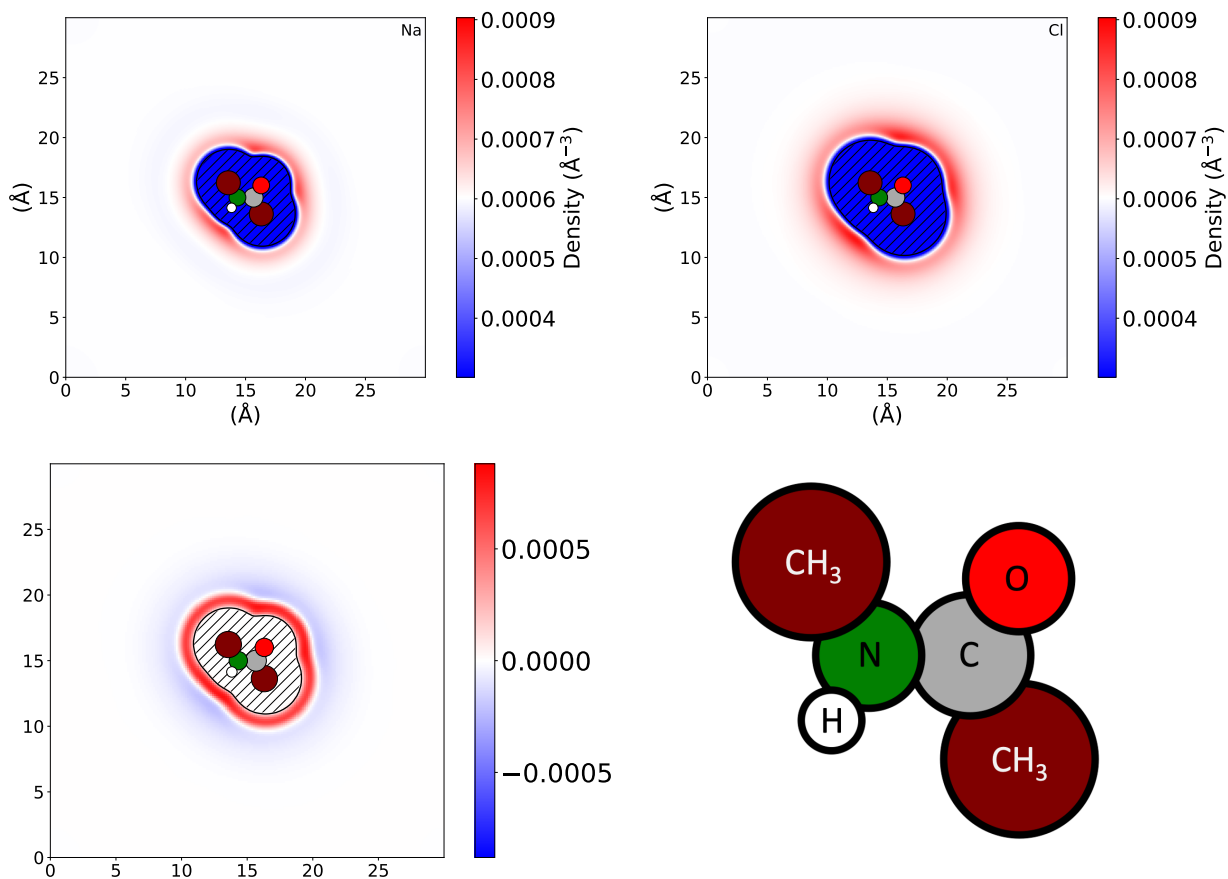

Figure 1. Slices of density in the plane of the NMA neutral molecule. The top panels display the sodium density (left) and the chloride density (right). The bottom panels show the charge density (left), defined as the difference between the sodium density and the chloride density.
